# Supplementary material for: Diffusive scaling of the Kob-Andersen model in $\mathbb{Z}^d$
Source: arXiv:1904.11078 ancillary file (2019-10-28)
Supplement: Supplementary file 1 [file appendix.pdf]

In this appendix we will prove Proposition 3.18 by constructing $T$-step moves and concatenating them to obtain the result.

## Definitions

We start by a few definitions that we will use in this construction.

**Definition 1.** Fix two directions $e, e' \in \{\pm e_1, \dots, \pm e_d\}$. Then the $(e,e')$-reflection of a site $x \in [\ell_1] \times \cdots \times [\ell_d]$ is the site $R_{e,e'}x$ of $[\ell_1] \times \cdots \times [\ell_d]$ given by

$$R_{e,e'}x = x - \langle e, x\rangle e - \langle e', x\rangle e' + \langle e, x\rangle e' + \langle e', x\rangle e \bmod (\ell_1, \dots, \ell_d)$$

for $e \neq -e'$, and

$$R_{e,e'}x = x - 2\langle e, x\rangle e$$

for $e = -e'$. This is an isometry that sends the vector $e$ to $e'$.

**Definition 2.** Fix $\ell_1, \dots, \ell_d$, and consider the box $B = [\ell_1] \times \cdots \times [\ell_d]$. Let $\eta \in \{0,1\}^B$. We define the notion of $(k,d)$-framed in the directions $\vec{e}_1, \dots, \vec{e}_d$

*Case* 1. For $k = 1$ we say that the box is $(k,d)$-framed if the site $(1, \dots, 1)$ is empty.

*Case* 2. For $d = k-1$ the box is $(k,d)$-framed when it is entirely empty.

*Case* 3. For $d \geq k > 1$ the box is framed when the first face$\{1\} \times [\ell_2] \times \cdots \times [\ell_d]$ is $(k, d-1)$-framed in the directions $\vec{e}_2, \dots, \vec{e}_d$, and each of the faces $\{m\} \times [\ell_2] \times \cdots \times [\ell_d]$, $m = 2, \dots, d$ is $(k-1, d-1)$-framed in the directions $\vec{e}_2, \dots, \vec{e}_d$.

Being framed in other directions (given by permutations of $\pm\vec{e}_1, \dots, \pm\vec{e}_d$) is defined by isometry, that is, $B$ is framed in the directions $\vec{e}'_1, \dots, e'_d$ for the configuration $\eta$ if $R_{e_1 e'_1} \dots R_{e_d e'_d} B$ is framed in the direction $\vec{e}_1, \dots, \vec{e}_d$ for the configuration $\eta'$ defined as

$$\eta'(x) = \eta\left(R_{e_1,\zeta e_1}x, \dots, R_{e_d,\zeta e_d}x\right).$$

**Example 3.** For $k = 2$, $d = 2$ a box is framed if its bottom line and leftmost column are empty. For $k = 2$, $d = 3$ a box is framed if the three edges touching the box's corner are empty. For $k = 3$,$d = 3$ a box is framed if the three faces touching the corner are empty.

**Proposition 4.** *The box* $[\ell_1] \times \cdots \times [\ell_d]$ *is* $(k,d)$*-framed in the directions* $\vec{e}_1, \dots, \vec{e}_d$ *for* $\eta \in \{0,1\}^{[\ell]^d}$ *iff every* $k-1$ *dimensional face containing the corner* $(1, \dots, 1)$ *is empty. That is, if* $x = (x_1, \dots, x_d)$ *satisfies*

$$\#\{1 \leq \alpha \leq d \,:\, x_\alpha = 1\} \geq d - k + 1 \tag{0.1}$$

*then* $\eta(x) = 0$. *In particular, being framed does not depend on permutations of* $\vec{e}_1, \dots, \vec{e}_d$, *but only on their signs.*

*Proof.* By induction. For $k=1$ the box is always framed iff the site $(1,\ldots,1)$ is empty, which is exactly the condition given in equation (0.1). For $d=k-1$ equation (0.1) is satisfied for all $x$, therefore the box must be entirely empty. For $d\geq k>1$ equation (0.1) is satisfied iff:

(1) $x_1=1$ and $\#\{2\leq\alpha\leq d\,:\,x_\alpha=1\}\geq(d-1)-k+1$,
(2) $x_1\neq1$ and $\#\{2\leq\alpha\leq d\,:\,x_\alpha=1\}\geq(d-1)-(k-1)+1$.

The first part describes equation (0.1) for the $(d-1,k)$-frameness of $\{1\}\times[\ell_2]\times\cdots\times[\ell_d]$, and the second corresponds to the $(d-1,k-1)$-frameness of each of the faces $\{m\}\times[\ell_2]\times\cdots\times[\ell_d]$, $m=2,\ldots,d$. □

**Definition 5.** Fix $\ell_1,\ldots,\ell_d$ and $\eta\in\Omega_\Lambda$. We say that the box $[\ell_1]\times\cdots\times[\ell_d]$ is $(d,k)$-frameable for $\eta$ if it is connected by legal FA$k$f moves in the box to a framed configuration in the directions $\vec{e}_1,\ldots,\vec{e}_n$.

It will sometime be useful to use the convention that boxes are always $(0,d)$-frameable.

**Definition 6.** Fix $\ell_1,\ldots,\ell_d$, and consider the box $[\ell_1]\times\cdots\times[\ell_d]$. We say that the box is $(k,d)$-almost good for the configuration $\eta$ if all $d-1$ dimensional faces contained in it are $(k-1,d-1)$-frameable for $\eta$. The box is good for $\eta$ if it is almost good for all configurations $\eta'$ that differ from $\eta$ by at most one site. For $k=1$ all boxes are good.

**Example 7.** For $k=2$,$d=2$ a box is good if every column and every line contain at least two empty sites. For $k=2$, $d=3$ a box is good if each 2 dimensional section contains at least two empty sites. For $k=3$, $d=3$ a box is good if each 2 dimensional section contains at least two empty sites in each row and in each column, and at least two non-intersecting rows or columns are empty.

Recall the definition of the loss of information of a move.

*Observation* 8. Let $M$ be a $T$-step move taking place in $V$. Then the loss of $M$ is at most the number of sites in $V$.

**Definition 9.** Fix a $T$-step move $M$ taking place in $V\subseteq\Lambda$, $\eta\in\mathrm{Dom}M$, and a sequence of permutation $(\sigma_0,\ldots,\sigma_T)$ on $V$, such that $\sigma_{t-1}^{-1}\sigma_t$ is either the identity or a nearest neighbors transposition for all $t\in[T]$. We say that $(\sigma_0,\ldots,\sigma_T)$ is compatible with $M\eta$ if for all $t\leq T$ and $x\in\Lambda$

$$M_t\eta\left(x\right)=\eta\left(\sigma_t x\right).$$

We say that $M\eta$ and the permutation $\sigma$ are compatible if there exists such a sequence with $\sigma_T=\sigma$. If the sequence $(\sigma_0,\ldots,\sigma_T)$ does not depend on $\eta$ we say that $M\eta$ and $\sigma$ are deterministically compatible.

*Observation* 10. Let $M$ be a $T$-step $\Lambda$, and assume that it is deterministically compatible with a permutation $\sigma$. Then $\text{Loss}M = 0$.

*Observation* 11. Fix a $T$-step move $M$ taking place in $V \subseteq \Lambda$. Let $\sigma$ be a random permutation compatible with $M$, i.e., for all $\eta \in \text{Dom}M$ the permutation $\sigma(\eta)$ is compatible with $M\eta$. Then there exists a $T'$ step move $M'$ with the same domain that is also compatible with $\sigma$, and $T' = |V|!$. If $\sigma$ is deterministic and $M$ is deterministically compatible with $\sigma$, than $M'$ will also be deterministically compatible with $\sigma$.

*Proof.* There could only be $|V|!$ unique permutations on $V$, so any sequence $(\sigma_0, \ldots, \sigma_T)$ of length $T \geq T'$ contains two equal permutations $\sigma_t = \sigma_s$ for $t < s$. It could then be shortened by removing the entries $t+1, \ldots, s$. Continue this procedure until $T \leq T'$ and pad it to obtain a $T'$ time move. □

**Definition 12.** Let $M^1$ be a $T_1$-step move and $M_2$ a $T_2$-step move. Assume that for all $\eta \in \text{Dom}M^1$, the configuration $M^1_{T_1}\eta$ is in $\text{Dom}M^2$. Then the composition $M^2 \circ M^1$ will be a $(T_1 + T_2)$-step move with $\text{Dom}M^2 \circ M^1 = \text{Dom}M^1$, such that

$$\left(M^2 \circ M^1\right)_t \eta = \begin{cases} M^1_t \eta & t \leq T_1 \\ M^2_{t-T_1} M_{T_1} \eta & T_1 < t \leq T_2 \end{cases}.$$

*Observation* 13. Fix $M^1$ a $T_1$-step move and $M^2$ a $T_2$-step move. Then the loss of their composition, when it is defined, is

$$\text{Loss}M^2 \circ M^1 = \max\left\{\text{Loss}M^1, \text{Loss}_{T_1} M^1 + \text{Loss}M^2\right\}.$$

Another operation on moves is choosing one out of a set of moves for different values of $\eta$.

**Definition 14.** Let $M^1, \ldots, M^n$ be a sequence of $T$-step move. Fix a set $\mathcal{M} \subset \Omega_\Lambda$, and a choice function $h$ form $\mathcal{M}$ to $[n]$. Assume that for every $\eta \in \mathcal{M}$

$$\eta \in \text{Dom}M^{h(\eta)}.$$

Then we may define a $T$-step move $M$ with domain $\mathcal{M}$ such that

$$M_t \eta = M^{h(\eta)}_t \eta.$$

*Observation* 15. Consider a sequence $M^1, \ldots, M^n$ and a choice function $h$ as in the above definition, and let $M$ be the corresponding move. Then

$$\text{Loss}M \leq \log_2 n + \sup_{i \in [n]} \text{Loss}M^i.$$

We are now ready to construct some basic $T$-step moves, by recursion on $d$ and $k$, and using previously defined moves on smaller $d$ and $k$. Unless written otherwise, moves are assumed to be defined for the KA$k$f in $d$ dimensions.

**Proposition 16** (Framed exchange move)**.** *Fix $x_0 \in \Lambda$, $\ell_2, \dots, \ell_d$. Let $F_1 = x_0 + \{1\} \times [\ell_2] \times \cdots \times [\ell_d]$ and $F_2 = x_0 + \{2\} \times [\ell_2] \times \cdots \times [\ell_d]$. Then there exists a $T$-step move $M$ taking place in $F_1 \cup F_2$ satisfying the following properties:*

*(1) $T$ is polynomial in $\ell_2 \dots \ell_d$,*

*(2) $DomM = \{\eta \,|\, F_1$ is $(d-1,k)$-framed and $F_2$ is $(d-1,k-1)$-framed$\}$ (framed refers to the directions $\vec{e}_2, \dots, \vec{e}_d$),*

*(3) $LossM = 0$,*

*(4) In the final state the two faces $F_1$ and $F_2$ are exchanged – for all $\eta \in DomM$*

$$M_T \eta\,(x) = \begin{cases} \eta(x + \vec{e}_\alpha) & x \in F_1 \\ \eta(x - \vec{e}_\alpha) & x \in F_2 \end{cases}.$$

*Moreover, $M$ is deterministically compatible with the permutation that exchanges $F_1$ and $F_2$.*

*By isometry this could also be defined for all other orientations. In the following we will refer to this move as the $(k,d)$ framed exchange move of the faces $F_1$ and $F_2$. We denote $T$ by $T^{k,d}_{fEx}(\ell_1, \dots, \ell_d)$.*

**Proposition 17** (Sliding move)**.** *Fix $x_0 \in \Lambda$, $\ell_1, \dots, \ell_d$ and $x \in [\ell_1] \times \cdots \times [\ell_d]$. Let $B = x_0 + [\ell_1] \times \cdots \times [\ell_d]$. Then there exists a $T^{k,d}$-step move $M$ taking place in $B$ satisfying the following properties:*

*(1) $T$ is polynomial in $\ell_2 \dots \ell_d$,*

*(2) $DomM = \{\eta \,|\, B$ is $(k,d)$-framed in the directions $\vec{e}_1, \dots, \vec{e}_d\}$,*

*(3) $LossM = 0$,*

*(4) $M$ is deterministically compatible with a permutation $\sigma$ that satisfies the following properties:*

*(a) $\sigma$ sends the $(k-1)$ dimensional faces containing the site $(1, \dots, 1)$ to the faces containing the site $x$. In particular, in the final state all $k-1$ dimensional face containing the site $x$ are empty.*

*(b) $\sigma$ fixes the sites in $x_0 + x + \mathbb{N}^d$, i.e., the sites that are strictly greater than $x_0 + x$ coordinate by coordinate.*

*By isometry this could also be defined for all other orientations. In the following we will refer to this move as the $(k,d)$ sliding move of the frame of $B$ into $x$. We denote $T$ by $T^{k,d}_{Sld}(\ell_1, \dots, \ell_d)$.*

**Proposition 18.** *Fix $x_0 \in \Lambda$, and let $M_1$ be a $T_1$-step move taking place in $x_0 + \{2\} \times [\ell_2] \times \cdots \times [\ell_d]$ for the KA$(k-1)$f dynamics in dimension $d-1$. Then there exits a $T$-step move $M$ taking place in $x_0 + \{1,2\} \times [\ell_2] \times \cdots \times [\ell_d]$ for the KAkf dynamics satisfying the following properties:*

*(1) $T = 2T^{k,d-1}_{Sld}\, T_1$,*

*(2)* $DomM = DomM_1 \cap \{\eta : x_0 + \{1\} \times [\ell_2] \times \cdots \times [\ell_d]$ *is* $(k, d-1)$ *-framed*$\}$,

*(3)* $LossM = LossM_1$,

*(4) If* $M_1$ *is compatible with a permutation* $\sigma$ *than* $M$ *is also compatible with* $\sigma$*. Moreover, if* $M_1$ *is deterministically compatible with* $\sigma$ *than* $M$ *will also be deterministically compatible with* $\sigma$*.*

*By isometry this could also be defined for all other orientations. In the following we will refer to this move as the application of* $M_1$ *on the face* $x_0 + \{2\} \times [\ell_2] \times \cdots \times [\ell_d]$ *with the help of the face* $x_0 + \{1\} \times [\ell_2] \times \cdots \times [\ell_d]$*.*

From now on, in order to simplify notation, we only consider $\ell_1 = \cdots = \ell_d = \ell$.

**Proposition 19** (Framing move)**.** *Fix* $x_0 \in \Lambda$ *and* $\zeta_1, \dots, \zeta_d \in \{+, -\}$*. Then there exists a* $T$*-step move* $M$ *taking place in* $x_0 + [\ell]^d$ *satisfying the following properties:*

*(1) For* $k = 1$ *the time* $T \leq dl$*, and for* $k \geq 2$ *it is bounded by* $T \leq 2^{\ell^d}$*,*

*(2)* $DomM = \left\{\eta : \text{the box } x_0 + [\ell]^d \text{ is } (d,k)\text{-frameable}\right\}$,

*(3) For* $k = 1$ $LossM \leq d \log \ell$ *and for* $k \geq 2$ $LossM \leq \ell^d$*.*

*(4) In the final state the box* $x_0 + [\ell]^d$ *is framed in the directions* $\zeta_1 e_1, \dots, \zeta_d e_d$*.*

*In the following we will refer to this move as the framing move of the box* $x_0 + [\ell]^d$ *in the directions* $\zeta_1 e_1, \dots, \zeta_d e_d$*. We denote* $T$ *by* $T_{Fr}^{k,d}(\ell_1, \dots, \ell_d)$*.*

In some cases we will need to frame boxes will smaller loss of information.

**Proposition 20** (Information saving framing move)**.** *Fix* $x_0 \in \Lambda$ *and* $\zeta_1, \dots, \zeta_d \in \{+, -\}$*. Then there exists a* $T$*-step move* $M$ *taking place in* $x_0 + [\ell]^d$ *satisfying the following properties:*

*(1) For* $k = 1$ *and* $k = 2$ *the time* $T$ *is bounded by a polynomial in* $\ell$*, and for* $k \geq 3$ $T \leq 2^{\ell^d}$*,*

*(2)* $DomM = \left\{\eta : x_0 + \{1\} \times [\ell]^{d-1} \text{ is } (d-1,k)\text{-framed and } x_0 + [\ell]^d \text{ is } (d,k) \text{ almost good}\right\}$,

*(3) For* $k = 1$ $LossM \leq d \log \ell$*, for* $k = 2$ $LossM \leq d^2 \ell \log \ell$*, and for* $k \geq 3$ $LossM \leq \ell^d$*,*

*(4) In the final state the box* $x_0 + [\ell]^d$ *is framed in the directions* $\zeta_1 e_1, \dots, \zeta_d e_d$*.*

*In the following we will refer to this move as the information saving framing move of the box* $x_0 + [\ell]^d$ *in the directions* $\zeta_1 e_1, \dots, \zeta_d e_d$*. We denote* $T$ *by* $T_{Fr}^{k,d}(\ell_1, \dots, \ell_d)$*.*

**Proposition 21** (Permutation move)**.** *Fix* $x_0 \in \Lambda$ *and a permutation* $\sigma$ *of the sites in* $x_0 + [\ell]^d$*. Assume that* $\sigma$ *fixes the frame defined as the set of sites satisfying 0.1. Then there exists a* $T$*-step move* $M$ *taking place in* $x_0 + [\ell]^d$ *satisfying the following properties:*

*(1)* $T$ *is polynomial in* $\ell$*,*

*(2)* $DomM = \left\{\eta \,|\, \text{the box } x_0 + [\ell]^d \text{ is framed in the directions } e_1, \dots, e_d\right\}$,

*(3)* $LossM = 0$*,*

*(4) The permutation* $\sigma$ *is deterministically compatible with* $M$*.*

*By isometry this could also be defined for boxes framed in all other directions. In the following we will refer to this move as the permutation move that applies* $\sigma$ *to* $x_0 + \{2, \ldots, \ell\}^d$. *We denote* $T$ *by* $T^{k,d}_{Per}$.

**Proposition 22** (Framed reflection move)**.** *Fix* $x_0 \in \Lambda$ *and* $e, e' \in \{\pm e_1, \ldots, \pm e_d\}$. *Then there exists a* $T$*-step move* $M$ *taking place in* $x_0 + [\ell]^d$ *satisfying the following properties:*

*(1)* $T$ *is polynomial in* $\ell$,
*(2)* $DomM = \left\{\eta \,|\, \text{the box } x_0 + [\ell]^d \text{ is framed in the directions } \vec{e}_1, \ldots, \vec{e}_d\right\}$,
*(3)* $LossM = 0$
*(4) It the final state the box* $x_0 + [\ell]^d$ *is reflected according to* $e, e'$:

$$M_T\eta\,(x) = \eta\,(R_{e,e'}x)\,.$$

*Moreover, the move is deterministically compatible with the permutation that sends* $x_0 + x$ *to* $x_0 + R_{e,e'}x$

*In the following we will refer to this move as the* $(k, d)$ *framed reflection move of* $x_0 + [\ell]^d$ *in the directions* $e, e'$. *We denote* $T$ *by* $T^{k,d}_{fRef}$.

**Proposition 23** (Reflection move)**.** *Fix* $x_0 \in \Lambda$ *and* $e, e' \in \{\pm e_1, \ldots, \pm e_d\}$. *Then there exists a* $T$*-step move* $M$ *taking place in* $x_0 + [\ell]^d$ *satisfying the following properties:*

*(1) For* $k = 1$ *and* $k = 2$ *the time* $T$ *is bounded by a polynomial in* $\ell$, *and for* $k \geq 3$ $T \leq 2^{\ell^d} \times$ *polynomial in* $\ell$,
*(2)* $DomM = \left\{\eta \,|\, \text{the box } x_0 + [\ell]^d \text{ is } (k, d) \text{ almost good and } x_0 + \{1\} \times [\ell]^{d-1} \text{ is } (d-1, k)\text{-framed}\right\}$,
*(3)* $Loss_T M = 0$,
*(4) For* $k = 1$ $LossM \leq d \log \ell$, *for* $k = 2$ $LossM \leq d^2 \ell \log \ell$, *and for* $k \geq 3$ $LossM \leq \ell^d$,
*(5) It the final state the box* $x_0 + [\ell]^d$ *is reflected according to* $e, e'$:

$$M_T\eta\,(x) = \eta\,(R_{e,e'}x)\,.$$

*That is, the move is compatible with the permutation that sends* $x_0 + x$ *to* $x_0 + R_{e,e'}x$

*In the following we will refer to this move as the* $(k, d)$ *reflection move of* $x_0 + [\ell]^d$ *in the directions* $e, e'$. *We denote* $T$ *by* $T^{k,d}_{Ref}$.

**Proposition 24** (Jump move)**.** *Fix* $x_0 \in \Lambda$, $e \in \{\pm e_1, \ldots, \pm e_d\}$ *and* $x^* = \left(x^*_1, \ldots, x^*_{d-1}\right) \in [\ell]^{d-1}$. *Let* $\alpha$ *be such that* $e \in \{\pm e_\alpha\}$ *and* $x^*_e = x_0 + \left(x^*_1, \ldots, x^*_{\alpha-1}, 0, x^*_\alpha, \ldots, x^*_{d-1}\right)$. *Then there exists a* $T$*-step move* $M$ *taking place in* $x_0 + [\ell]^{\alpha-1} \times \{-1, 0, 1\} \times [\ell]^{d-\alpha}$ *satisfying the following properties:*

*(1) For* $k = 2$ *and* $k = 3$ *the time* $T$ *is bounded by a polynomial in* $\ell$, *and for* $k \geq 4$ $T \leq 2^{\ell^d} \times$ *polynomial in* $\ell$,

*(2) For a fixed configuration $\eta$, let $\eta^*$ be the configuration that equals $\eta$ for $x \notin \{x_e^* + e, x_e^* - e\}$ and 1 for $x \in \{x_e^* + e, x_e^* - e\}$. With this notation,*

$$\begin{aligned} DomM &= \Big\{\eta \,|\, \textit{the face } x_0 + [\ell]^{\alpha-1} \times \{1\} \times [\ell]^{d-\alpha} \textit{ and the face} \\ &\quad x_0 + [\ell]^{\alpha-1} \times \{-1\} \times [\ell]^{d-\alpha} \textit{ are } (k-1, d-1) \textit{ frameable for } \eta^*, \\ &\quad \textit{and the face } x_0 + [\ell]^{\alpha-1} \times \{0\} \times [\ell]^{d-\alpha} \textit{ is } (k, d-1) \textit{ framed}\Big\}, \end{aligned}$$

*(3) For $k = 2$ $LossM \le 2d \log \ell$, for $k = 3$ $LossM \le 2d^2 \ell \log \ell$, and for $k \ge 4$ $LossM \le 2\ell^d$.*

*(4) It the final state*

$$M_T\eta\,(x) = \begin{cases} \eta\,(x_e^* + e) & x = x_e^* - e \\ \eta\,(x_e^* - e) & x = x_e^* + e\ , \\ \eta\,(x) & \textit{otherwise} \end{cases}$$

*i.e., $M\eta$ is compatible with the permutation that exchanges $x_e^* + e$ and $x_e^* - e$.*

*In the following we will refer to this move as the jump move of the site $x_e^* - e$ to $x_e^* + e$. We denote $T$ by $T_{Jmp}^{k,d}$.*

For the construction of the next moves we will use the notion of geometric paths, which are the same as the paths of the previous sections but with some extra information.

**Definition 25.** A geometric path of length $n$ is a sequence $i_1, \dots, i_n \in \left(\mathbb{Z}_\ell^d\right)^n$, together with two directions $e_{\text{in}}^{(1)}, e_{\text{out}}^{(n)} \in \{\pm e_1, \dots, \pm e_d\}$, such that $i_{\tau+1} - i_\tau \in \{\pm e_1, \dots, \pm e_d\}$ for all $\tau < n$. We will denote, at each step $\tau$, $e_{\text{in}}^{(\tau)} = i_\tau - i_{\tau-1}$ and $e_{\text{out}}^{(\tau)} = i_\tau - i_{\tau+1}$. We say that the geometric path is good if for a configuration $\eta$ of the box $B_{i_\tau}$ is good for all $\tau$, and super-good if it is good and the face $\ell i_1 + R_{e_1, e_{\text{in}}^{(1)}}\left(\{1\} \times [\ell]^{d-1}\right)$ is $(k, d-1)$-framed.

We will also need to keep track of the time a move spends at some fixed box

**Definition 26.** Consider a $T$-step move $M$ and some set $V \subset \mathbb{Z}^d$. Then the time $M$ spends in $V$ for a configuration $\eta$ is

$$\mathcal{T}_{M,\eta}^V = \{t \in [T] \,:\, \exists x \in B_j \text{ such that } M_t\eta\,(x) \ne M_{t+1}\eta\,(x)\}\,.$$

We denote $\mathcal{T}_M^V = \cup_{\eta \in \text{Dom}M} \mathcal{T}_{M,\eta}^V$. When $V = B_i$ for some $i \in \mathbb{Z}_\ell^d$ we will use the notation $\mathcal{T}_{M,\eta}^{(i)}$ and $\mathcal{T}_M^{(i)}$.

**Proposition 27.** *Fix a geometric path $i_1, \dots, i_n$ with directions $e_{in}^{(1)}, e_{out}^{(n)}$, and $x^* \in [\ell]^{d-1}$. Let $x_{e_{in}^{(1)}}^* = \ell i_1 + R_{e_1, e_{in}^{(1)}}(2, x^*)$ (in analogy with Proposition 24) and $x_{e_{out}^{(n)}}^* = \ell i_n + R_{e_1, e_{out}^{(n)}}(2, x^*)$. Then there exists a $T$-step move $M$ taking place in $\bigcup_{\tau=1}^n B_{i_\tau}$ satisfying the following properties:*

*(1) $T = n \times$ polynom in $\ell$ for $k = 1$ or $k = 2$, and $T \le 2^{\ell^d} \times$ polynomial in $\ell$ for $k \ge 3$,*

(2) $DomM = \{\eta : \text{the path is super-good}\}$,
(3) For $k=1$ $LossM \le 2d\log\ell$, for $k=2$ $LossM \le 2d^2\ell\log\ell$, and for $k\ge 3$ $LossM \le 2\ell^d$,
(4) $\left|\mathcal{T}_M^{(j)}\right|$ is bounded by $\frac{2T}{n}$, uniformly for all $j \in \mathbb{Z}_\ell^d$,
(5) The path $i_n,\dots,i_1$ with directions $e_{out}^{(n)}, e_{in}^{(1)}$ is super-good for the configuration $M_T\eta$.
(6) There exists a permutation $\sigma$, independent of $\eta$, such that
   (a) $\sigma$ is compatible with $M\eta$ for all $\eta \in DomM$,
   (b) $\sigma x^*_{e_{in}^{(1)}} = x^*_{e_{out}^{(n)}}$.

**Proposition 28** (Swap move)**.** *Fix $i \in \mathbb{Z}_\ell^d$ and $x^* = (x_1^*, x_2^*, \dots, x_d^*) \in [\ell]^d$. Then there exists a $T$-step move $M$ taking place in $B_i \cup Q_i$ satisfying the following properties:*

(1) $T$ = polynom in $\ell$,
(2) For every box $j \in Q_i$, we write $j = \sum_{\alpha\in d} c_\alpha \vec{e}_\alpha$ for $c_\alpha \in \{0,1\}$. Let $c'_\alpha = \begin{cases} 1 & c_\alpha = 1 \\ -1 & c_\alpha = 0 \end{cases}$.
   Then

$$DomM = \{\eta : \text{For ever } j \in Q_i \text{ the box } B_j \text{ is } (k,d)\text{-framed in the directions } c'_1\vec{e}_1,\dots,c'_d\vec{e}_d\},$$

(3) $LossM = 0$,
(4) $M$ is deterministically compatible with the permutation that swaps the sites $\ell i + x^*$ and $\ell(i+e_1) + (2, x_2^*, \dots, x_d^*)$.

*In the following we will refer to this move as the swap move of $\ell i + x^*$ and $\ell(i+e_1) + (2, x_2^*, \dots, x_d^*)$.*

We are finally ready to show how to flip a single site.

**Proposition 29.** *Fix a geometric path $i_1,\dots,i_n,i_{n+1}$ with directions $e_{in}^{(1)}, e_{out}^{(n)}$ such that $i_1 - e_{in}^{(1)} \notin \Lambda_\ell$. Fix $x^* \in [\ell]^d$. Set $i = i_{n+1}$. Then there exists a $T$-step move $M$ taking place in $\bigcup_{\tau=1}^n B_{i_\tau} \cup Q_i$ satisfying the following properties:*

(1) $T = n \times$ polynom in $\ell$ for $k=1$ or $k=2$, and $T = 2^{\ell^d} \times$ polynomial in $\ell$ for $k \ge 3$,
(2) $DomM = \{\eta : \text{the path } i_1,\dots,i_n \text{ is good and the boxes } Q_i \text{ are good}\}$,
(3) For $k=1$ $LossM \le 10d\log\ell$, for $k=2$ $LossM \le 10d^2\ell\log\ell$, and for $k\ge 3$ $LossM \le 10\ell^d$,
(4) $E(M) \le C_{k,d}\ell^{k-1}$, where $C_{k,d}$ is a positive constant that may depend on $k$ and $d$,
(5) $\left|\mathcal{T}_M^{(j)}\right|$ is bounded by $\frac{2T}{n}$, uniformly for all $j \in \mathbb{Z}_\ell^d$,
(6) $M_T\eta = \eta^{\ell i + x^*}$, i.e., the site $\ell i + x^*$ is flipped.

Constructing the moves

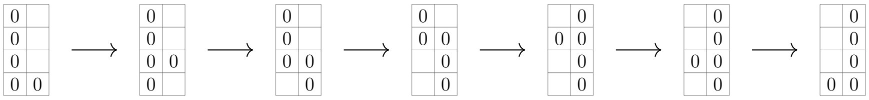

FIGURE 0.1. The framed exchange move for $k = d = 2$

**The framed exchange move (Proposition 16).** Assume WLOG $x_0 = 0$, $\ell_2 \le \cdots \le \ell_d$, and take $\eta \in \mathrm{Dom}M$. Note that the definition of $\mathrm{Dom}M$ is equivalent to the requirement that the box $[2] \times [\ell_2] \times \cdots \times [\ell_d]$ is $(k, d)$-framed in the directions $\vec{e}_1, \dots, \vec{e}_d$.

For $k = 1$, the KA-1f dynamics is the unconstrained one, so we may simply exchange the two frames site by site.

For $\ell_2 = 2$, by Proposition 4, the box $[2] \times \{1\} \times [\ell_3] \times \cdots \times [\ell_d]$ is $(k, d-1)$ framed – being framed does not depend on the order in which we take the directions, therefore $[2] \times [\ell_2] \times \cdots \times [\ell_d]$ is $(k, d)$-framed also in the directions $\vec{e}_2, \vec{e}_1, \vec{e}_3, \dots, \vec{e}_d$. We can thus use Proposition 18 in order to apply $(d-1, k-1)$ moves to $[2] \times \{2\} \times [\ell_3] \times \cdots \times [\ell_d]$. We also know that $[2] \times \{2\} \times [\ell_3] \times \cdots \times [\ell_d]$ is $(k-1, d-1)$ framed, so $\eta$ is in the domain of the $(k-1, d-1)$ frame exchange move that exchanges $\{1\} \times \{2\} \times [\ell_3] \times \cdots \times [\ell_d]$ and $\{2\} \times \{2\} \times [\ell_3] \times \cdots \times [\ell_d]$. Proposition 18 thus allows us to exchange these two faces. In order to finish we need to exchange $\{1\} \times \{1\} \times [\ell_3] \times \cdots \times [\ell_d]$ and $\{2\} \times \{1\} \times [\ell_3] \times \cdots \times [\ell_d]$. This could be done using the $(k, d-1)$ framed exchange move – $[2] \times \{1\} \times [\ell_3] \times \cdots \times [\ell_d]$ is $(k, d-1)$ framed, so $\eta$ is indeed in its domain.

If $\ell_2 > 2$, we start by exchanging the faces $[2] \times \{1\} \times [\ell_3] \times \cdots \times [\ell_d]$ and $[2] \times \{2\} \times [\ell_3] \times \cdots \times [\ell_d]$. This could be done since these two faces are in the domain of the $(k, d)$-frame exchange move, with faces whose smallest side is 2. For this new configuration, will will first consider the sites of $[2] \times \{1\} \times [\ell_3] \times \cdots \times [\ell_d]$, and then the sites of $[2] \times \{2, \dots, \ell_2\} \times [\ell_3] \times \cdots \times [\ell_d]$.

The face $[2] \times \{2\} \times [\ell_3] \times \cdots \times [\ell_d]$ is now $(k, d-1)$ framed, so we will use Proposition 18 in order to apply $(d-1, k-1)$ moves to $[2] \times \{1\} \times [\ell_3] \times \cdots \times [\ell_d]$. The face $[2] \times \{1\} \times [\ell_3] \times \cdots \times [\ell_d]$ is $(k-1, d-1)$-framed in the directions $\vec{e}_1, e_3, \dots, \vec{e}_d$. That is, $\{1\} \times \{1\} \times [\ell_3] \times \cdots \times [\ell_d]$ is $(k-1, d-2)$-framed and $\{2\} \times \{1\} \times [\ell_3] \times \cdots \times [\ell_d]$ is $(k-2, d-2)$-framed. This allows us to exchange these two faces using the $(k-1, d-2)$ framed exchange move.

The box $[2] \times \{2, \dots, \ell_2\} \times [\ell_3] \times \cdots \times [\ell_d]$ is $(k, d)$-framed in the directions $\vec{e}_1, \dots, \vec{e}_d$, so we apply (by induction) the $(k, d)$ framed exchange move on it with a smaller value of $\ell_2$.

Finally, we exchange back the two faces $[2] \times \{1\} \times [\ell_3] \times \cdots \times [\ell_d]$ and $[2] \times \{2\} \times [\ell_3] \times \cdots \times [\ell_d]$, and this conclude the construction of the move. See Figure 0.1.

**The frame sliding move (Proposition 17).** Assume WLOG $x_0 = 0$, and set $x = (x_1, \dots, x_d)$. Use the framed exchange move $x_1$ times in order to move the face $\{1\} \times [\ell_2] \times \cdots \times [\ell_d]$ to $\{x_1\} \times [\ell_2] \times \cdots \times [\ell_d]$. Consider now the box $\{x_1, \dots, \ell_1\} \times [\ell_2] \times \cdots \times [\ell_d]$. It is framed in the directions $\vec{e}_1, \dots, \vec{e}_d$, so we can apply the sliding move by induction into the point $x$. Similarly,

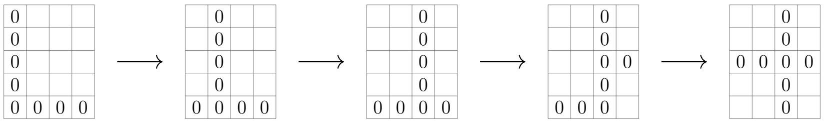

FIGURE 0.2. The frame sliding move for $k = d = 2$

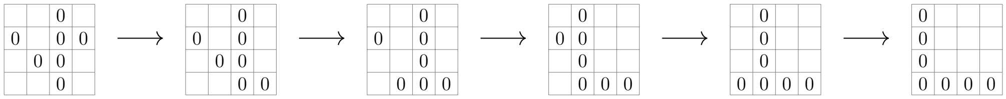

FIGURE 0.3. The box framing move for $k = d = 2$

the box $[x_1] \times [\ell_2] \times \cdots \times [\ell_d]$ is framed in the directions $-\vec{e}_1, \ldots, \vec{e}_d$, and again we can apply the sliding move into the point $x$. See Figure 0.2.

**Performing $(k-1, d-1)$ moves near a framed face (Proposition 18).** For each exchange of $M$ of two sites $x, y$, start by sliding the frame of $x_0 + \{1\} \times [\ell_2] \times \cdots \times [\ell_d]$ to a the site $x - \vec{e}_1$. Then both $x$ and $y$ get an extra empty neighbor.

**Framing a box (Proposition 19).** Assume WLOG that $\zeta_1 = \cdots = \zeta_d = +$. Start with $k = 1$, i.e., the unconstrained case. For $x \in x_0 + [\ell]^d$ we will use a $T$-step move $M^x$ whose domain is $\{\eta : x \text{ is empty}\}$, deterministically compatible with a permutation $\sigma$ that satisfies $\sigma x = x_0 + (1, \ldots, 1)$. Since the dynamics is not constrained, we can construct such a move with $T = d\ell$. We then use the choice function defined for $\eta \in \mathrm{Dom} M$, that assigns to $\eta$ the move $M^x$, for $x \in x_0 + [\ell_1] \times \cdots \times [\ell_d]$ that is empty for $\eta$ (when ambiguous we take the minimal one in some arbitrary order). This function is well defined since $\eta \in \mathrm{Dom} M$ means (for $k = 1$) that at least one of the sites in $x_0 + [\ell]^d$ is empty. We can then define $M$ as in Definition 14, and 15 completes the proof for this case.

For $k > 1$, by definition of frameability there exists a move that frames the box. The bounds on the time and on the loss come from the fact that there are at most $2^{\ell^d}$ configurations in the box.

See Figure 0.3.

**Information saving framing (Proposition 20).** Assume WLOG that $x_0 = 0$ and $\zeta_1 = \cdots = \zeta_d = +$. Note that for $\eta \in \mathrm{Dom} M$ the box $x_0$ is frameable, so it suffices to consider $k = 2$.

The face $\{1\} \times [\ell]^{d-1}$ is framed, therefore by Proposition 18 we can apply $(d-1, 1)$ moves to $\{2\} \times [\ell]^{d-1}$. This face is $(d-1, 1)$-frameable, so we may apply the framing move in order to frame it. Then we use the framed exchange move and exchange $\{1\} \times [\ell]^{d-1}$ with $\{2\} \times [\ell]^{d-1}$. In the same way we frame $\{3\} \times [\ell]^{d-1}$ and exchange it with $\{2\} \times [\ell]^{d-1}$, until framing $\{\ell\} \times [\ell]^{d-1}$. We can then exchange back $\{\ell - 1\} \times [\ell]^{d-1}$ with $\{\ell - 2\} \times [\ell]^{d-1}$ and so on until it is back to $\{1\} \times [\ell]^{d-1}$. By 13 and the fact that $(d-1, 1)$ framing has loss $d \log \ell$ the result follows.

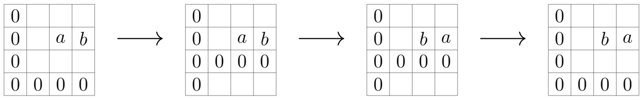

FIGURE 0.4. The permutation move for $k = d = 2$

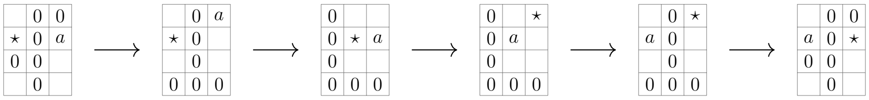

FIGURE 0.5. The jump move for $k = d = 2$

**The permutation move (Proposition 21).** Assume first that $\sigma$ is a transposition that exchanges two neighboring sites, without loss of generality $x = (x_1, \dots, x_d)$ and $y = x + \vec{e}_d$. If $k = 1$ we can simply exchange the two sites. Consider now $k \geq 2$. We know that $x$ is not on the frame of $[\ell]^d$, so at least $k$ of its coordinates are different than 1. We can assume that one of these coordinates is the first one, i.e., $x_1 > 1$. We will then slide the frame of $[\ell]^d$ to the point $(x_1 - 1, 1, \dots, 1)$, without changing the sites of $[x_1, \ell] \times [\ell]^d$. After this move, the face $\{x_1 - 1\} \times [\ell]^{d-1}$ is $(k, d-1)$ framed, so we may apply $(k-1, d-1)$ moves to the face $\{x_1\} \times [\ell]^{d-1}$. Note that $\{x_1\} \times [\ell]^{d-1}$ is $(k-1, d-1)$ framed and both $x$ and $y$ are contained in it. Moreover, $x$ and $y$ are not on the frame of $\{x_1\} \times [\ell]^{d-1}$, so we can use the lower dimensional permutation move to exchange them. Then rewind the sliding move finishes the construction.

Finally, we note that every transposition can be written as a product of at most $2d\ell$ nearest-neighbor transposition, and every permutation can be written as the sum of at most $\ell^d \log \ell^d$ permutations. This concludes the proof. See Figure 0.4.

**The framed reflection move (Proposition 22).** Assume without loss of generality $x_0 = 0$. First, slide the frame into the point $R_{e,e'}(1, \dots, 1)$. The frame of the resulting configuration is indeed the reflected frame, and for the other site we can use Proposition 21.

**The reflection move (Proposition 23).** In order to reflect a box, we start by framing it in the direction $\vec{e}_1, \dots, \vec{e}_d$. We then apply a framed reflection, and finally unwrap the framing move that we have applied in the beginning.

**The jump move (Proposition 24).** Start by framing the face $x_0 + [\ell]^{\alpha-1} \times \{0\} \times [\ell]^{d-\alpha}$. Then, by Proposition 18 we can also frame the faces $x_0 + [\ell]^{\alpha-1} \times \{\pm 1\} \times [\ell]^{d-\alpha}$ for $\eta^*$. When framing these faces, $x_e^* - \vec{e}_1$ and $x_e^* + \vec{e}_1$ could change position, so we denote by $y - \vec{e}_1$ and $y' + \vec{e}_1$ their new positions. We can now exchange $x_0 + [\ell]^{\alpha-1} \times \{0\} \times [\ell]^{d-\alpha}$ and $x_0 + [\ell]^{\alpha-1} \times \{-1\} \times [\ell]^{d-\alpha}$ using the framed exchange, permute $x_e'$ with $y' + \vec{e}_1$ with the permutation move, and exchange again $x_0 + [\ell]^{\alpha-1} \times \{0\} \times [\ell]^{d-\alpha}$ and $x_0 + [\ell]^{\alpha-1} \times \{-1\} \times [\ell]^{d-\alpha}$. All that is left is to wind back the framing moves and we are done. See Figure 0.5.

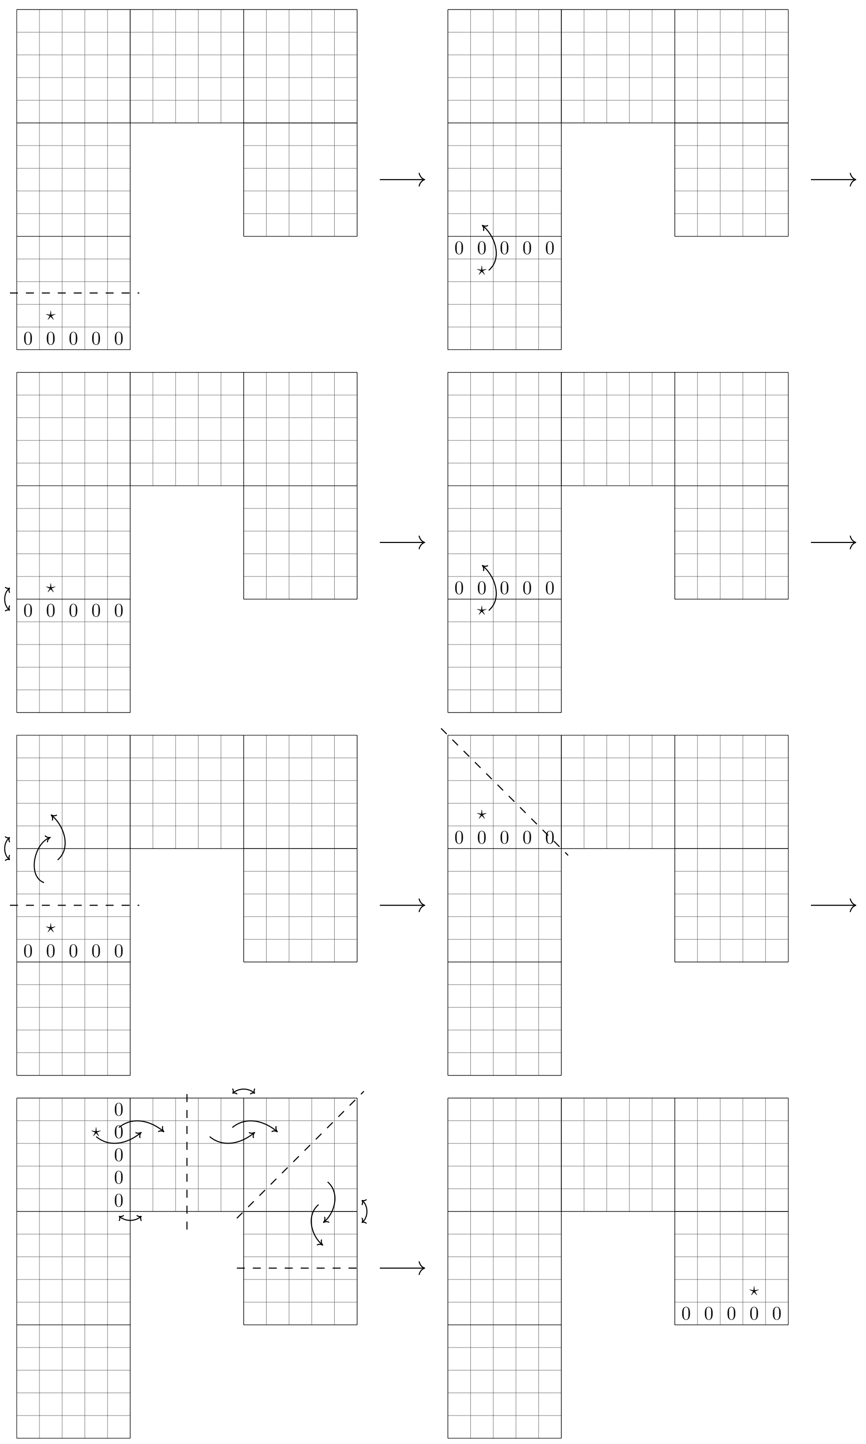

FIGURE 0.6. Propagating a site along a path for $k = d = 2$

**Propagating a site along a path (Proposition 27).** We construct this move by induction over $n$. For $n = 1$ the reflection move of the box $B_{i_1}$ in the directions $e_{\text{in}}, e_{\text{out}}$ will give the result.

For $n > 1$, propagate the site along the first $n-1$ boxes. We can then apply the jump move swapping $x^*_{e^{(n-1)}_{\text{out}}}$ with $x^*_{e^{(n)}_{\text{in}}}$. This gives the required move. See Figure 0.6.

**The swap move (Proposition 28).** Note that for $\eta \in \text{Dom}M$ the box $i + [\ell+1]^d$ is framed in the directions $-\vec{e}_1, \ldots, -\vec{e}_d$. We can thus apply the permutation move in order to move the site $\ell i + x^*$ to $\ell i + (\ell, x^*_2, \ldots, x^*_d)$. Then the jump move allows us to swap $\ell i + (\ell, x^*_2, \ldots, x^*_d)$ with $\ell i + (\ell + 2, x^*_2, \ldots, x^*_d) = \ell(i + e_1) + (2, x^*_2, \ldots, x^*_d)$, and then applying the inverse permutation finishes the construction.

**Flipping a site (Proposition 29).** The first step is to frame the boxes of $Q_i \setminus \{i + \vec{e}_1\}$. By creating $O\left(\ell^{k-1}\right)$ zeros on the boundary, we can frame the first face of the box $i_1$ making the path super-good. Then we apply Proposition 27 $d-1$ times (with arbitrary $x^*$), and framing $Q_i \setminus \{i + \vec{e}_1\}$ in the directions required by Proposition 27. We can do that since by adding boxes in $Q_i$ to the path $i_1, \ldots, i_n$ we can obtain a super-good path that reaches each of the boxes in $Q_i$. We then use the boundary condition and set the site $\ell i_1 + R_{e_1, e^{(1)}_{\text{in}}}(2, x^*_2, \ldots, x^*_d)$ to have the occupation value $1 - \eta(\ell i + x^*)$. Then propagate the site along the path using Proposition 27 and swap it with $\ell i + x^*$ using Proposition 28. We now roll back everything, and the proof is finished.
